# Supplementary material for: Double Adaptive Stochastic Gradient Optimization
Source: arXiv:1811.02525 source file (2018-11-06)
Supplement: Supplementary file 1 [file section_appendix_lr_selection.tex]

%%%%%%%%%%%%%%%%%%%%%%%%%%%%%%%%%%%%%%%%%%%%%%%%%%%%%%%%%%%%
\begin{table}[ht]
\begin{threeparttable}
    \centering
    \scriptsize
    \caption{Training Accuracy after first 500 Steps for the MNIST dataset}
    \begin{tabular}{l c c c c c c c c c c c} 
    \hline
    \hline
     &  &  \multicolumn{10}{c}{\textbf{Learning Rates}} \\
    \textbf{Optimizer} & & 0.001& 0.002& 0.003 & 0.004 & 0.005 & 0.006 & 0.007 & 0.008&  0.009& 0.010  \\
    \cline{1-1} \cline{3-12}
      & &  &   &   &   &   &   &   &   &   &    \\
     ADAM & & 0.9327 &  0.9528 &  0.9611 &  0.9625 &  0.9654 &  0.9678 &  0.9694 &  0.9700 &  0.9705 &  0.9710  \\
     \hline
     AMSGrad & & 0.9282 &  0.9494 &  0.9500 &  0.9547 &  0.9576 &  0.9596 &  0.9609 &  0.9621 &  0.9633 &  0.9638 \\
     \hline 
     DASGrad & & 0.9362 &  0.9534 &  0.9634 &  0.9675 &  0.9655 &  0.9643 &  0.9604 &  0.9617 &  0.9585 & 0.9676 \\
     \hline
     \hline
     & & \multicolumn{10}{c}{\textbf{Learning Rates}} \\
    \textbf{Optimizer} & & 0.01& 0.02& 0.03 & 0.04 & 0.05 & 0.06 & 0.07 & 0.08&  0.09& 0.10 \\
    \cline{1-1} \cline{3-12}
      &  &  &   &   &   &   &   &   &   &   &    \\
     \textsc{Adam} & & \textbf{0.9710} & 0.9378& 0.8932 & 0.8317 & 0.8137 & 0.7683 & 0.7497 & 0.7411&  0.7278& 0.7260  \\
     \textsc{AMSGrad} & &  \textbf{0.9638} & 0.9324& 0.8838& 0.8395& 0.8094& 0.7724& 0.7585& 0.7398& 0.7267& 0.7283 \\
     \hline 
     \textsc{DASGrad} & &  \textbf{0.9676} & 0.9383 & 0.9073 & 0.8837 & 0.8582 & 0.8630 & 0.8485 & 0.8307 & 0.8028 & 0.8051 \\
    \hline
      &  &  &   &   &   &   &   &   &   &   &    \\
    \end{tabular}
    \begin{tablenotes}
    \scriptsize
    \item \textbf{Note: } For the grid search of learning rate parameter for the MNIST dataset, we first explore the interval $[0.01, 0.1]$, after seeing that the best learning rate parameters for all three optimization methods are 0.1, we explore $[0.001, 0.01]$. In the end, the best learning rate for all three optimization methods are 0.01. For each learning rate, for each optimizer, we run 20 random seeds and report the average resulting accuracy after 500 steps, on 50000 training data points in the MNIST dataset.
    \end{tablenotes}
    \end{threeparttable}
\end{table}

%Accuracies (averages) for AMSGrad:
%[0.9282500058412552, 0.9494500070810318, 0.9500499963760376, 0.9547999978065491, 0.9576999932527542, 0.9596499979496003, 0.9609500050544739, 0.9621500134468078, 0.9633500039577484, 0.9638999998569489]
%Accuracies (averages) for Adam:
%[0.9327500015497208, 0.9528499960899353, 0.9611999988555908, 0.9625, 0.9654000103473663, 0.9678500056266784, 0.9694000005722045, 0.9700500011444092, 0.970550000667572, 0.9710500061511993]
%Accuracies (averages) for DASGrad:
%[0.9362500011920929, 0.9534500002861023, 0.9634999990463257, 0.967550003528595, 0.9655500024557113, 0.9643999934196472, 0.9604500025510788, 0.9617000013589859, 0.9585000067949295, 0.9676500022411346]

%%%%%%%%%%%%%%%%%%%%%%%%%%%%%%%%%%%%%%%%%%%%%%%%%%%%%%%%%%%%

%%%%%%%%%%%%%%%%%%%%%%%%%%%%%%%%%%%%%%%%%%%%%%%%%%%%%%%%%%%%
\begin{table}[ht]
\begin{threeparttable}
\centering
\scriptsize
\caption{Training Accuracy after first 500 Steps for the IMDB dataset}
\begin{tabular}{l c c c c c c c c c c c} 
\hline
\hline
 &  &  \multicolumn{10}{c}{\textbf{Learning Rates}} \\
\textbf{Optimizer} & & 0.001& 0.002& 0.003 & 0.004 & 0.005 & 0.006 & 0.007 & 0.008&  0.009& 0.010  \\
\cline{1-1} \cline{3-12}
  & &  &   &   &   &   &   &   &   &   &    \\
 \textsc{Adam} & & 0.8955& 0.9072& 0.9111& 0.9130& \textbf{0.9135}& 0.9134& 0.9129& 0.9119& 0.9108& 0.9099   \\
 \hline
 \textsc{AMSGrad} & &0.8935& 0.9055& 0.9102& 0.9125& 0.9135& \textbf{0.9136} & 0.9130& 0.91234& 0.9117& 0.9109\\
 \hline 
 \textsc{DASGrad} & & 0.8975& 0.9147& 0.9243& 0.9314& 0.9359& 0.9399& 0.9429& 0.9455& 0.9474&  0.9494\\
\hline
\hline
 &  &  \multicolumn{10}{c}{\textbf{Learning Rates}} \\
\textbf{Optimizer} & & 0.01& 0.02& 0.03 & 0.04 & 0.05 & 0.06 & 0.07 & 0.08&  0.09& 0.10  \\
\cline{1-1} \cline{3-12}
  & &  &   &   &   &   &   &   &   &   &    \\
 \textsc{Adam} & & 0.9099 & 0.8970  & 0.8836 &  0.8775 &  0.8706 &    0.8567 &  0.8535 &  0.8497 &   0.8447 &  0.8369  \\
 \hline
 \textsc{AMSGrad} & & 0.9109 & 0.8988 & 0.8884 & 0.8812&  0.8741 &   0.8671 &   0.8633 &  0.8518 &  0.8488 &  0.8489\\
 \hline 
 \textsc{DASGrad} & & 0.9494 & \textbf{0.9571}  &  0.9548&  0.9516 &  0.9445 & 0.9342  &  0.9288 &  0.9229 & 0.9217 &  0.9144 \\
 \hline
  &  &  &   &   &   &   &   &   &   &   &    \\
\end{tabular}
    \begin{tablenotes}
    \scriptsize
    \item \textbf{Note:} For the grid search of learning rate parameter for the IMDB dataset, we first explore the interval $[0.01, 0.1]$, after seeing that the best learning rate parameters for ADAM and AMSGrad are 0.1, we explore $[0.001,0.01]$. In the end, the best learning rate for ADAM is 0.005, the best rate for AMSGrad is 0.006, and the best rate for DASGrad is 0.02. For each learning rate, for each optimizer, we run 20 random seeds and report the average resulting accuracy after 500 steps, on 20000 training data points in the IMDB dataset.
    \end{tablenotes}
\end{threeparttable}
\end{table}

\begin{table}[ht]
    \begin{threeparttable}
    \centering
    \scriptsize
    \caption{Number of Iterations to Solve CartPole Environment for Double Q Linear Agent}
    \begin{tabular}{l c c c c c c c c c c c} 
    \hline
    \hline
     &  &  \multicolumn{10}{c}{\textbf{Learning Rates}} \\
    \textbf{Sampling} & & 1e-5& 2e-5& 3e-5 & 4e-5 & 5e-5 & 6e-5 & 7e-5 & 8e-5&  9e-5& 1e-4\\
    \cline{1-1} \cline{3-12}
      & &  &   &   &   &   &   &   &   &   &    \\
     %Uniform  &  & 41450& 40150& 41350& 39750& 41200& 41650& 41600& \textbf{38300}& 41300& 40200 \\
     %\hline
     TD Error &  & 41,450 & 42,200 & 41,150 & 41,100& 41,600& \textbf{38,950}& 41,650& 40,900& 41,500& 42,150 \\
     \hline 
     DASGrad  &  & 41,650& 40,900& \textbf{39,050} & 39,450& 39,700& 50,200& 59,300& 41,800& 41,950& 41,750 \\
     \hline
      &  &  &   &   &   &   &   &   &   &   &    \\
    \end{tabular}
    \begin{tablenotes}
    \scriptsize
    \item \textbf{Note:} For the grid search of learning rate parameter for training a double Q linear network agent in the CartPole-v0 environment, we explore the interval $[1e-5 - 1e-4]$. In the end, the best rate for the TD error based prioritized experience replay is $6e-5$, and the best rate for DASGrad prioritized experience replay is $3e-5$. The buffer size we used is 5,000. For each learning rate, for each sampling method, we average over 20 random seeds, to obtain the average number of iterations needed for the average past 100 episode reward to reach 200. For each of the 20 random seed, for each sampling method and each learning rate, we run a max of 50,000 iterations, with an initial exploration rate of 100\% and a final exploration rate of 2\%, decaying over 60\% of the total iterations, and testing every 1,000 iterations. 
    \end{tablenotes}
    \end{threeparttable}
\end{table}

%%%%%%%%%%%%%%%%%%%%%%%%%%%%%%%%%%%%%%%%%%%%%%%%%%%%%%%%%%%%
